# Supplementary material for: MF-Box: Multi-fidelity and multi-scale emulation for the matter power spectrum
Source: arXiv:2306.03144 source file (2023-10-04)
Supplement: Supplementary file 1 [file appendix.tex]

\section{Emulation using SRGAN}

\begin{figure}
    \includegraphics[width=\columnwidth]{images/boxsize/dgmgp_srgan_dmonly_50_3.pdf}
    \caption{A deep graphical Gaussian process model with an additional low-fidelity information source, super-resolution GAN.}
 \end{figure}
